# Supplementary material for: Quiet Triggers, Loud Footprints: A Tri-Space Measurement Study of Backdoor Stealthiness
Source: arXiv:2610.19947 source file (2026-10-14)
Supplement: Supplementary file 1 [file appendix.tex]

% \section{Stealthiness Metric Baselines}
% \label{sec:baselines}
% %To put our results on CIFAR-10 in Tables~\ref{tab:input-stealthiness-all},~\ref{tab:results_feature_resnet18}, and~\ref{tab:uclc-tac} into perspective, we evaluate the stealthiness metrics on clean data and models in this section.

% \textbf{Input-space metrics.} For all metrics, we have measured the distance between each data sample $i$ and $i + 1~(\text{mod}~N)$, where $N$ is the length of the testing dataset, and averaged the measurements over all $i$. The results are given in \autoref{tab:baseline_input_cifar10}. We observe that with the exception of the $l_\infty$ and SAM metrics, all backdoor attacks on CIFAR-10 perform better than the baseline. It makes sense that the perturbation induced by the backdoor triggers is generally smaller than the distance between two completely different images.

% \begin{table}
%     \centering
%     \footnotesize
%     \caption{Input-space stealthiness baselines on CIFAR-10.}
%     \label{tab:baseline_input_cifar10}
%     \renewcommand{\arraystretch}{1.15}
%     \begin{tabular}{rcc}
%         \toprule
%         Metric & Ideal value & Baseline measurement\\
%         \midrule
%         $l_1 \downarrow$ & 0 & 862\\
%         $l_2 \downarrow$ & 0 & 18.8\\
%         $l_\infty \downarrow$ & 0 & 0.845\\
%         MSE $\downarrow$ & 0 & 0.121\\
%         PSNR $\uparrow$ & $\infty$ & 9.18\\
%         SSIM $\uparrow$ & 1 & 0.0393\\
%         LPIPS $\downarrow$ & 0 & 0.211\\
%         IS $\downarrow$ & 0 & 4.32\\
%         pHash $\uparrow$ & 100 & 51.1\\
%         SAM $\downarrow$ & 0 & 0.216\\
%         \bottomrule
%     \end{tabular}
% \end{table}

% \textbf{Feature-space metrics.} In feature space, we use a different methodology for each metric. For the silhouette score, we use $k$-means with $k=2$ to divide the feature representations of clean data samples into two clusters, following the approach of the AC defense~\cite{chen2018ac}. These features are extracted from the data by a benign ResNet18 model. To measure a baseline for DSWD, we have split the testing dataset into two halves and computed the distance between them. 

% From \autoref{tab:baseline_feature_resnet18_cifar10}, we observe that the silhouette score baseline is higher than the measurements on a small number of backdoored ResNet18 models. This suggests that these backdoored models are unlikely to be detected by the AC defense. For DSWD, on the other hand, the baseline is lower than the measurements of all backdoored models.

% \begin{table}
%     \centering
%     \footnotesize
%     \caption{Feature-space stealthiness baselines of backdoored ResNet18 models on CIFAR-10.}
%     \label{tab:baseline_feature_resnet18_cifar10}
%     \renewcommand{\arraystretch}{1.15}
%     \begin{tabular}{rcc}
%         \toprule
%         Metric & Ideal value & Baseline measurement\\
%         \midrule
%         SS $\downarrow$ & -1 & 0.366\\
%         DSWD $\downarrow$ & 0 & 0.0675\\
%         \bottomrule
%     \end{tabular}
% \end{table}

% \textbf{Parameter-space metrics.} In this space, our baseline methodology also differs between the metrics. For UCLC, we simply evaluate the metric on the benign ResNet18 model. For TAC, we adopt a similar methodology as the input-space baseline: we compare the feature-space representations between each data sample $i$ and $i + 1~(\text{mod}~N)$. 

% In Table~\ref{tab:baseline_parameter_resnet18_cifar10}, we see that the UCLC baseline is lower than the majority of the backdoored ResNet18 model measurements on CIFAR-10. The Grond models are the largest exception, which can be explained by UCLC being minimized during training. The baseline suggests that most backdoored models could be effectively distinguished from a benign model by the CLP defense~\cite{zheng2022clp} with the right choice for the hyperparameter $u$. However, it must be taken into account that our measurement is only based on the neuron with the maximum UCLC, and a backdoor may be injected into multiple neurons. For TAC, the baseline is lower than the measurement for all backdoored models.

% \begin{table}[htbp]
%     \centering
%     \footnotesize
%     \caption{Parameter-space stealthiness baselines of backdoored ResNet18 models on CIFAR-10.}
%     \label{tab:baseline_parameter_resnet18_cifar10}
%     \begin{tabular}{l c c}
%         \toprule
%         Metric & Ideal Value & Baseline Measurement \\
%         \midrule
%         UCLC $\downarrow$ & 0 & 6.09 \\
%         TAC $\downarrow$ & 0 & 1.46 \\
%         \bottomrule
%     \end{tabular}
% \end{table}



% \textbf{New metrics.} We have not measured a baseline for the CDBI and TUP metrics proposed in this paper. This is because these metrics rely more on the presence of poisoned data or backdoored models than the metrics previously discussed in this section. CDBI assumes one of the two clusters in the t-SNE embedding is poisoned, and divides it into smaller subclusters depending on the data samples' original class. TUP reduces the influence of a trigger's input-space perturbation by calculating the ratio between the TAC for a backdoored and clean model.

% \section{Detailed Analysis of SAM Measurements}
% \label{sec:sam_analysis}
% We now analyze the two peculiarities of the SAM measurements mentioned in Section~\ref{sec:experimental_results} by focusing on the CIFAR-10 measurements.

% \textbf{BadNets versus DFBA.} With most other metrics, these two attacks are considered similarly stealthy on CIFAR-10. However, SAM considers BadNets to be significantly stealthier. The root cause of this behavior is shown in Figure~\ref{fig:sam_per_pixel}. It reveals that for the BadNets attack, the average SAM measurement is approximately uniform across all trigger pixels. In contrast, the DFBA trigger exhibits significant variance, with certain pixels registering substantially higher measurements than others. 

% \begin{figure}[t]
%     \centering
%     \includegraphics[width=0.95\linewidth]{img/sam_per_pixel.png}
%     \caption{SAM comparison for BadNets, DFBA, WaNet, and BppAttack on CIFAR-10. The average measurements are shown for each individual pixel in the $32 \times 32$ poisoned images.}
%     \label{fig:sam_per_pixel}
% \end{figure} 

% Cross-referencing these measurements with the CIFAR-10 DFBA trigger in Figure~\ref{fig:cifar10_dfba} indicates that the elevated SAM values correspond to the colored pixels within the trigger pattern, whereas the lower measurements align with the black and white pixels. This discrepancy implies that, on average, the angular divergence in the vector representations between a trigger pixel and the original image pixel it replaces is more pronounced for colored pixels. Consequently, the aggregate SAM measurement for BadNets is lower than for DFBA, attributable to its exclusive use of black and white pixels.

% \begin{figure}[t]
%     \centering
%     \includegraphics[width=0.3\linewidth]{img/cifar10_dfba.png}
%     \caption{CIFAR-10 image poisoned with the DFBA trigger.}
%     \label{fig:cifar10_dfba}
% \end{figure} 

% The underlying cause for this spectral behavior is rooted in the pixel value distributions across color channels. For the colored pixels in the DFBA trigger, individual color channels are set to their maximum or minimum values independently, creating a vector that points in a direction divergent from the natural image distribution. Conversely, in the black and white pixels, all three color channels are set uniformly to either the minimum or maximum value, resulting in a vector aligned with the axis of the normalized color space. As seen in Table~\ref{tab:normalization}, the average pixel in the CIFAR-10 dataset possesses similar values across its color channels, meaning its vector representation is directionally congruent with the uniform vectors of black and white pixels but incongruent with the imbalanced vectors of the colored pixels, thus explaining the measured spectral angle differences.

% The underlying cause for this spectral behavior is rooted in the pixel value distributions across color channels. For the colored pixels in the DFBA trigger, individual color channels are set to their maximum or minimum values independently, creating a vector that points in a direction divergent from the natural image distribution. Conversely, in the black and white pixels, all three color channels are set uniformly to either the minimum or maximum value, resulting in a vector aligned with the axis of the normalized color space. As seen in Table~\ref{tab:normalization}, the average pixel in the CIFAR-10 dataset possesses similar values across its color channels, meaning its vector representation is directionally congruent with the uniform vectors of black and white pixels but incongruent with the imbalanced vectors of the colored pixels, thus explaining the measured spectral angle differences.

% \textbf{WaNet versus BppAttack.} SAM considers WaNet to be stealthier than BppAttack, whereas the opposite is true for all other metrics on CIFAR-10. The per-pixel SAM measurements in Figure~\ref{fig:sam_per_pixel} demonstrate considerable variability for WaNet, but remarkable consistency for BppAttack. The uniform measurement for BppAttack is logically consistent, as its method of reducing the color depth of the entire image applies a global transformation that affects all pixels equally on average. For WaNet, the high variance suggests that the warping-based perturbation does not affect all pixels uniformly; it is hypothesized that the SAM measurement peaks in regions where the warping distortion is most severe, though the trigger's imperceptibility makes direct confirmation challenging. Nevertheless, it can be concluded that WaNet achieves a superior aggregate stealth score from SAM because a significant proportion of its trigger pixels induce only a very minor angular deviation, thereby lowering its average measurement.

% \section{Other Model Architectures}
% \label{sec:other-arch}

% The attack performance of the three model architectures on CIFAR-10 is provided in Table~\ref{tab:attack-performance-3arch}.
% Since the training data remains unchanged across different model architectures, we do not include input space evaluation for other architectures.
% In addition, we provide the feature space metrics (SS and DSWD) for VGG16 and ViT-Small in Table~\ref{tab:feature-vgg-vit}. 
% Parameter space evaluation for VGG16 is provided in Table~\ref{tab:parameter-vgg}.
% Parameter space evaluation for ViT is not offered because UCLC and TAC are designed based on the convolutional channel for CNN architectures, which is not compatible with the ViT architecture.


% \begin{table}[htbp]
%     \centering
%     \footnotesize
%     \setlength{\tabcolsep}{2.8pt}
%     \caption{Performance of three architectures on CIFAR-10.}
%     \label{tab:attack-performance-3arch}
%     \begin{tabular}{l *{6}{c}}
%     \toprule
%     Attack & \multicolumn{2}{c}{ResNet18} & \multicolumn{2}{c}{VGG16} & \multicolumn{2}{c}{ViT-Small} \\
%     \cmidrule(lr){2-3} \cmidrule(lr){4-5} \cmidrule(lr){6-7}
%     ~ & BA & ASR & BA & ASR & BA & ASR \\
%     \midrule
%     Benign     & 94.7 & --   & 93.50 & --    & 80.62 & --    \\
%     Badnet     & 94.5 & 100  & 93.45 & 100   & 80.94 & 100   \\
%     Blended    & 94.3 & 99.8 & 93.43 & 99.66 & 81.10 & 98.96 \\
%     Wanet      & 93.4 & 98.5 & 88.94 & 99.40 & 79.00 & 22.12 \\
%     Bpp        & 94.4 & 99.8 & 93.08 & 59.52 & 79.29 & 3.47  \\
%     Adap-P     & 93.9 & 30.1 & 93.87 & 28.73 & 79.21 & 23.35 \\
%     Adap-B     & 94.0 & 53.9 & 94.08 & 64.58 & 79.93 & 83.51 \\
%     DFST       & 95.0 & 100  & --    & --    & --    & --    \\
%     Narcis.    & 94.4 & 100  & 93.50 & 100   & 79.68 & 100   \\
%     Grond      & 94.7 & 92.9 & 93.20 & 85.00 & 80.60 & 100   \\
%     DFBA       & 94.3 & 100  & 93.20 & 100   & --    & --    \\
%     \bottomrule
%     \end{tabular}
% \end{table}



% % Bpp, Adap-patch have low SS and DSWD scores, because their ASRs are not good.

% \begin{table}[htbp]
%     \centering
%     \footnotesize
%     \setlength{\tabcolsep}{5pt}
%     \caption{Feature-space stealthiness of backdoored VGG16 and ViT-Small models on CIFAR-10.}
%     \label{tab:feature-vgg-vit}
%     \begin{tabular}{l *{4}{c}}
%     \toprule
%     Attack & \multicolumn{2}{c}{VGG16} & \multicolumn{2}{c}{ViT-Small} \\
%     \cmidrule(lr){2-3} \cmidrule(lr){4-5}
%     ~ & SS & DSWD & SS & DSWD \\
%     \midrule
%     Badnet  & .515 & 2.784 & .263 & 2.719 \\
%     Blended & .524 & 2.712 & .433 & 2.637 \\
%     Wanet   & .398 & 1.978 & .195 & .290  \\
%     Bpp     & .330 & 1.171 & .174 & .022  \\
%     Adap-P  & .257 & .742  & .220 & .609  \\
%     Adap-B  & .243 & 1.284 & .296 & 1.203 \\
%     Narcis. & .459 & 3.360 & .467 & 3.431 \\
%     Grond   & .317 & 2.340 & .375 & 2.114 \\
%     DFBA    & --   & 3.900 & --   & --    \\
%     \bottomrule
%     \end{tabular}
% \end{table}



% \begin{table}[htbp]
%     \centering
%     \footnotesize
%     \setlength{\tabcolsep}{2.5pt}
%     \caption{Parameter-space stealthiness of backdoored VGG16 models trained on three datasets.}
%     \label{tab:parameter-vgg}
%     \begin{tabular}{l c *{6}{c}}
%     \toprule
%     Model & PR & \multicolumn{2}{c}{CIFAR-10} & \multicolumn{2}{c}{CIFAR-100} & \multicolumn{2}{c}{Imagenette} \\
%     \cmidrule(lr){3-4} \cmidrule(lr){5-6} \cmidrule(lr){7-8}
%     ~ & ~ & UCLC & TAC & UCLC & TAC & UCLC & TAC \\
%     \midrule
%     Benign    & -- & 7.75 & -- & 4.63 & -- & 4.66 & -- \\
%     Narcissus & 5/0.7/5$^*$ & 13.5 & 1.39 & 4.74 & 1.98 & 6.67 & 1.89 \\
%     Grond     & 5/0.7/5$^*$ & 4.12 & .608 & 4.77 & 1.74 & 3.78 & 1.04 \\
%     DFBA      & -- & 20.7 & 5.67 & 15.7 & 13.0 & 19.1 & 58.3 \\
%     \bottomrule
%     \end{tabular}
% \end{table}

% \section{t-SNE Embeddings for ResNet18}
% \label{app:t-sne}

% The t-SNE feature space embeddings of the backdoored ResNet18 models on the CIFAR-10, CIFAR-100, Tiny-ImageNet, and Imagenette datasets are shown in Figures~\ref{fig:cifar-tsne},~\ref{fig:cifar100-tsne},~\ref{fig:tiny-tsne}, and~\ref{fig:imagenette-tsne}, respectively.





% \newcommand{\tsnefigurecifar}[4][0.003]{
% \begin{subfigure}[b]{0.3\textwidth}
%         \centering
%         \caption{#4}
%         \vspace{-0.25cm}
%         \includegraphics[width=0.49\linewidth]{tsne/#2/#3_p0.05/default.png}
%         \includegraphics[width=0.49\linewidth]{tsne/#2/#3_p#1/default.png}
%     \end{subfigure}
% }


% \captionsetup[subfigure]{labelformat=empty}
% \begin{figure*}[htbp]
%     \centering
%     % Row 1: Groups 1-3 (6 images total)
%     \tsnefigurecifar{resnet18_cifar10}{badnet}{BadNets}
%     \hfill
%     \tsnefigurecifar{resnet18_cifar10}{blended}{Blend}
%     \hfill
%     \tsnefigurecifar[0.02]{resnet18_cifar10}{wanet}{WaNet}
    
%     \vspace{-0.25cm} % Row spacing adjustment
    
%     % Row 2: Groups 4-6 (6 images total)
%     \tsnefigurecifar{resnet18_cifar10}{adaptive_patch}{Adaptive-Patch}
%     \hfill
%     \tsnefigurecifar{resnet18_cifar10}{adaptive_blend}{Adaptive-Blend}
%     \hfill
%     \tsnefigurecifar[0.02]{resnet18_cifar10}{bpp}{Bpp}
    
%     \vspace{-0.25cm}
    
%     % Row 3: Groups 7-9 (6 images total)
%     \tsnefigurecifar{resnet18_cifar10}{dfst}{DFST}
%     \hfill
%     \tsnefigurecifar{resnet18_cifar10}{narcissus}{Narcissus}
%     \hfill
%     \tsnefigurecifar{resnet18_cifar10}{grond}{Grond}
    
%     \vspace{-0.25cm}
    
%     \hspace{1cm}
%     \text{\small PR=0.05 \hspace{1cm} PR=0.003}
%     \hfill
%     \text{\small PR=0.05 \hspace{1cm} PR=0.003}
%     \hfill
%     \text{\small PR=0.05 \hspace{1cm} PR=0.003$^*$}
%     \hspace{1cm}
    
%     \caption{t-SNE feature space embeddings of backdoored models on the CIFAR-10 training dataset, poisoned with the specified poisoning rate (PR). Benign samples are
% colored \textcolor{blue}{blue}, while poisoned samples are colored \textcolor{red}{red}. *WaNet and Bpp use PR=0.02.}
%     \label{fig:cifar-tsne}
% \end{figure*}




% \newcommand{\tsnefigure}[5]{
% \begin{subfigure}[b]{0.32\textwidth}
%         \centering
%         \caption{#5}
%         \includegraphics[width=0.49\linewidth]{tsne/#1/#2_p#3/default.png}
%         \includegraphics[width=0.49\linewidth]{tsne/#1/#2_p#4/default.png}
%     \end{subfigure}
% }

% \captionsetup[subfigure]{labelformat=empty}
% \begin{figure*}[htbp]
%     \centering
%     % Row 1: Groups 1-3 (6 images total)
%     \tsnefigure{resnet18_cifar100}{badnet}{0.05}{0.003}{BadNets}
%     \hfill
%     \tsnefigure{resnet18_cifar100}{blended}{0.05}{0.003}{Blend}
%     \hfill
%     \tsnefigure{resnet18_cifar100}{wanet}{0.05}{0.003}{WaNet}
    
%     \vspace{-0.5cm} % Row spacing adjustment
    
%     % Row 2: Groups 4-6 (6 images total)
%     \tsnefigure{resnet18_cifar100}{bpp}{0.05}{0.003}{Bpp}
%     \hfill
%     \tsnefigure{resnet18_cifar100}{adaptive_patch}{0.05}{0.003}{Adaptive-Patch}
%     \hfill
%     \tsnefigure{resnet18_cifar100}{adaptive_blend}{0.05}{0.003}{Adaptive-Blend}
    
%     \vspace{-0.5cm}
    
%     % Row 3: Groups 7-9 (6 images total)
%     \tsnefigure{resnet18_cifar100}{dfst}{0.05}{0.003}{DFST}
%     \hfill
%     \tsnefigure{resnet18_cifar100}{narcissus}{0.007}{0.003}{Narcissus}
%     \hfill
%     \tsnefigure{resnet18_cifar100}{grond}{0.007}{0.003}{Grond}
    
%     \vspace{-0.5cm}
    
%     \hspace{1cm}
%     \text{\small PR=0.05 \hspace{1cm} PR=0.003}
%     \hfill
%     \text{\small PR=0.05 (0.007*) \hspace{0.5cm} PR=0.003}
%     \hfill
%     \text{\small PR=0.05 (0.007*) \hspace{0.5cm} PR=0.003}
%     \hspace{0.75cm}
    
%     \caption{t-SNE feature space embeddings of backdoored models on the CIFAR-100 training dataset, poisoned with the specified poisoning rate (PR). Benign samples are
% colored \textcolor{blue}{blue}, while poisoned samples are colored \textcolor{red}{red}. *The PRs for Narcissus and Grond are 0.007 and 0.003.}
%     \label{fig:cifar100-tsne}
% \end{figure*}


% \captionsetup[subfigure]{labelformat=empty}
% \begin{figure*}[htbp]
%     \centering
%     % Row 1: Groups 1-3 (6 images total)
%     \tsnefigure{resnet18_tiny}{badnet}{0.05}{0.003}{BadNets}
%     \hfill
%     \tsnefigure{resnet18_tiny}{blended}{0.05}{0.003}{Blend}
%     \hfill
%     \tsnefigure{resnet18_tiny}{wanet}{0.05}{0.003}{WaNet}
    
%     \vspace{-0.5cm} % Row spacing adjustment
    
%     % Row 2: Groups 4-6 (6 images total)
%     \tsnefigure{resnet18_tiny}{bpp}{0.05}{0.003}{Bpp}
%     \hfill
%     \tsnefigure{resnet18_tiny}{adaptive_patch}{0.05}{0.003}{Adaptive-Patch}
%     \hfill
%     \tsnefigure{resnet18_tiny}{adaptive_blend}{0.05}{0.003}{Adaptive-Blend}
    
%     \vspace{-0.5cm}
    
%     % Row 3: Groups 7-9 (6 images total)
%     \tsnefigure{resnet18_tiny}{dfst}{0.05}{0.003}{DFST}
%     \hfill
%     \tsnefigure{resnet18_tiny}{narcissus}{0.004}{0.003}{Narcissus}
%     \hfill
%     \tsnefigure{resnet18_tiny}{grond}{0.004}{0.003}{Grond}
    
%     \vspace{-0.5cm}
    
%     \hspace{1cm}
%     \text{\small PR=0.05 \hspace{1cm} PR=0.003}
%     \hfill
%     \text{\small PR=0.05 (0.004*) \hspace{0.5cm} PR=0.003}
%     \hfill
%     \text{\small PR=0.05 (0.004*) \hspace{0.5cm} PR=0.003}
%     \hspace{0.75cm}
    
%     \caption{t-SNE feature space embeddings of backdoored models on the Tiny-ImageNet training dataset, poisoned with the specified poisoning rate (PR). Benign samples are
% colored \textcolor{blue}{blue}, while poisoned samples are colored \textcolor{red}{red}. *The PRs for Narcissus and Grond are 0.004 and 0.003.}
%     \label{fig:tiny-tsne}
% \end{figure*}



% \captionsetup[subfigure]{labelformat=empty}
% \begin{figure*}[htbp]
%     \centering
%     % Row 1: Groups 1-3 (6 images total)
%     \tsnefigure{resnet18_imagenette}{badnet}{0.05}{0.003}{BadNets}
%     \hfill
%     \tsnefigure{resnet18_imagenette}{blended}{0.05}{0.003}{Blend}
%     \hfill
%     \tsnefigure{resnet18_imagenette}{wanet}{0.05}{0.003}{WaNet}
    
%     \vspace{-0.5cm} % Row spacing adjustment
    
%     % Row 2: Groups 4-6 (6 images total)
%     \tsnefigure{resnet18_imagenette}{bpp}{0.05}{0.003}{Bpp}
%     \hfill
%     \tsnefigure{resnet18_imagenette}{adaptive_patch}{0.05}{0.003}{Adaptive-Patch}
%     \hfill
%     \tsnefigure{resnet18_imagenette}{adaptive_blend}{0.05}{0.003}{Adaptive-Blend}
    
%     \vspace{-0.5cm}
    
%     % Row 3: Groups 7-9 (6 images total)
%     \tsnefigure{resnet18_imagenette}{dfst}{0.05}{0.003}{DFST}
%     \hfill
%     \tsnefigure{resnet18_imagenette}{narcissus}{0.05}{0.003}{Narcissus}
%     \hfill
%     \tsnefigure{resnet18_imagenette}{grond}{0.05}{0.003}{Grond}
    
%     \vspace{-0.5cm}
    
%     \hspace{1cm}
%     \text{\small PR=0.05 \hspace{1cm} PR=0.003}
%     \hfill
%     \text{\small PR=0.05 \hspace{1cm} PR=0.003}
%     \hfill
%     \text{\small PR=0.05 \hspace{1cm} PR=0.003}
%     \hspace{0.75cm}
    
%     \caption{t-SNE feature space embeddings of backdoored models on the Imagenette training dataset, poisoned with the specified poisoning rate (PR). Benign samples are
% colored \textcolor{blue}{blue}, while poisoned samples are colored \textcolor{red}{red}.}
%     \label{fig:imagenette-tsne}
% \end{figure*}



% \section{TAC Visualizations for ResNet18}
% \label{sec:tac-visualization}

% The TAC visualizations of the backdoored ResNet18 models on the CIFAR-10, CIFAR-100, and Imagenette datasets are shown in Figures~\ref{fig:cifar10-tac},~\ref{fig:cifar100-tac}, and~\ref{fig:imagenette-tac}, respectively. 
% The TAC measurements provided in Section~\ref{subsec:parameter-space-stealthiness} are taken from the neuron with maximum TAC in these visualizations. The visualizations themselves are inspired by~\cite[Figure 9]{xu2025grond}.

% \begin{figure*}
%     \centering
%     \includegraphics[width=\linewidth]{img/TAC_comparison_resnet18_cifar10.png}
%     \caption{Comparison of the trigger-activated change (TAC) values of each backdoor
% attack on CIFAR-10. In each plot, the \textcolor{red}{red} line shows the TAC values for a model
% backdoored with the specified attack and poisoning rate (PR), where applicable. The
% \textcolor{blue}{blue} line shows the TAC values for a benign model on the same inputs. Each TAC
% value belongs to one neuron in the model, and the neurons are sorted according to
% their TAC values for clearer visualization.}
%     \label{fig:cifar10-tac}
% \end{figure*} 


% \begin{figure*}
%     \centering
%     \includegraphics[width=\linewidth]{img/TAC_comparison_resnet18_cifar100.png}
%     \caption{Comparison of the trigger-activated change (TAC) values of each backdoor
% attack on CIFAR-100. In each plot, the \textcolor{red}{red} line shows the TAC values for a model backdoored with the specified attack and poisoning rate (PR), where applicable. The
% \textcolor{blue}{blue} line shows the TAC values for a benign model on the same inputs. Each TAC
% value belongs to one neuron in the model, and the neurons are sorted according to
% their TAC values for clearer visualization.}
%     \label{fig:cifar100-tac}
% \end{figure*} 


% \begin{figure*}
%     \centering
%     \includegraphics[width=\linewidth]{img/TAC_comparison_resnet18_imagenette.png}
%     \caption{Comparison of the trigger-activated change (TAC) values of each backdoor
% attack on Imagenette. In each plot, the \textcolor{red}{red} line shows the TAC values for a model backdoored with the specified attack and poisoning rate (PR), where applicable. The
% \textcolor{blue}{blue} line shows the TAC values for a benign model on the same inputs. Each TAC
% value belongs to one neuron in the model, and the neurons are sorted according to
% their TAC values for clearer visualization.}
%     \label{fig:imagenette-tac}
% \end{figure*} 
