# Supplementary material for: Quiet Triggers, Loud Footprints: A Tri-Space Measurement Study of Backdoor Stealthiness
Source: arXiv:2610.19947 source file (2026-10-14)
Supplement: Supplementary file 2 [file appendix_robustness.tex]

%%%%%%%%%%%%%%%%%%%%%%%%%%%%%%%%%%%%%%%%%%%%%%%%%%%%%%%%%%%%%%%%%%%%%%%%%%%%%%%%
% Appendix: Robustness, Uncertainty and Reproducibility Analyses
%
% Add to main.tex after the other appendices, e.g.:
%     \input{sections/appendix_robustness}
%
% Requires (all already loaded in main.tex): booktabs, tabularx, multirow,
% threeparttable, array, xcolor[table].
%%%%%%%%%%%%%%%%%%%%%%%%%%%%%%%%%%%%%%%%%%%%%%%%%%%%%%%%%%%%%%%%%%%%%%%%%%%%%%%%

\appendices
\section{Robustness, Uncertainty and Reproducibility}
\label{app:robustness}

The benchmark in Section~\ref{sec:benchmark_results} reports one trained realization per
configuration, which is the usual regime for backdoor benchmarks but leaves open how much of the
reported structure is attributable to training randomness, to the choice of target class, or to
implementation choices inside individual metrics. This appendix reports four analyses that bound
those effects. Appendix~\ref{app:rob:bootstrap} quantifies the uncertainty of the metric-agreement
analysis by resampling, including a cluster bootstrap that respects the dependence between
configurations sharing an attack. Appendix~\ref{app:rob:seeds} repeats training across random seeds
and target classes and recomputes every footprint metric. Appendix~\ref{app:rob:winners} retrains
the two attacks that hold the feature- and parameter-space minima five times at each of three
target classes and verifies the minima in every run.
Appendix~\ref{app:rob:cdbi} measures how far CDBI's rankings depend on the embedding it is computed
in. Appendix~\ref{app:rob:derived} recomputes the agreement analysis with metrics that are derived
by construction from other metrics removed.

Throughout this appendix, metrics are oriented as in Section~\ref{sec:metric_disagreement}: larger
values always denote larger measured footprints, and metrics for which higher is conventionally
better (PSNR, SSIM, pHash, CDBI) are inverted before any correlation is computed.

\subsection{Uncertainty of the Metric-Agreement Analysis}
\label{app:rob:bootstrap}

\paragraph{Motivation}
Section~\ref{sec:metric_disagreement} treats each backdoored ResNet18 configuration
(dataset~$\times$~attack~$\times$~poisoning rate) as one observation and reports Spearman
correlations over $N{=}76$ such observations. Two objections apply. First, no interval is attached
to the reported correlations, so it is unclear how much of the within-versus-across-space structure
would survive a different draw of configurations. Second, the observations are not independent:
eight of the $76$ rows are BadNets configurations that share a trigger and an implementation and
differ only in dataset and poisoning rate. An attack that is extreme under some metric therefore
displaces eight rows in the same direction rather than one, so the effective sample size is closer
to the number of attacks than to the number of configurations, and significance computed under an
independence assumption is optimistic.

\paragraph{Method}
We estimate percentile bootstrap $95\%$ confidence intervals from $2000$ resamples for each block
average of Table~\ref{tab:metric_correlation_blocks}, for the summary quantity
\emph{within-minus-cross-space agreement} (the mean of the three within-space block averages minus
the mean of the three cross-space block averages), and for four individual metric pairs of
interest. Three resampling schemes are used, in increasing order of conservatism with respect to the
dependence structure:

\begin{itemize}
\item \emph{configuration} --- resample the $76$ rows with replacement. This is the naive scheme and
      corresponds to the independence assumption criticized above.
\item \emph{attack cluster} --- resample the ten attacks with replacement, taking all configurations
      of a drawn attack together. An attack is either wholly present in a resample or wholly absent,
      so between-configuration dependence within an attack cannot inflate precision. This is the
      scheme we regard as authoritative.
\item \emph{dataset cluster} --- resample the four datasets with replacement, analogously.
\end{itemize}

Every scheme is applied both to all $76$ configurations and to the subset with
$\mathrm{ASR}\geq 60\%$ ($N{=}61$), so that the effect of excluding backdoors that were never
successfully implanted can be read off directly. Correlations are recomputed from scratch inside
each resample; block averages are formed by Fisher-$z$ transformation, averaging, and back
transformation.

\paragraph{Results}
Table~\ref{tab:app:bootstrap} reports the intervals. The within-versus-cross-space gap is
$+0.50$ with an attack-cluster interval of $[0.28, 0.62]$, and $+0.51$ with $[0.27, 0.64]$ on the
ASR-filtered subset; in neither case does the interval approach zero. The strongest individual
cross-space association, between $\ell_1$ input distortion and TUP, is $-0.69$ with an
attack-cluster interval of $[-0.80,-0.47]$, and strengthens to $-0.72$ under ASR filtering. The
input--parameter block average also strengthens under filtering, from $-0.24$ to $-0.33$, so
excluding failed backdoors reinforces rather than weakens the paper's central claim.

Two blocks are individually fragile under the most conservative resampling, and we report this
explicitly. The parameter--parameter block average, $+0.27$, has an attack-cluster interval of
$[-0.04, 0.52]$ that includes zero, as does the underlying UCLC--TAC pair
($+0.05$, $[-0.44, 0.50]$). This is consistent with the analysis in
Appendix~\ref{app:rob:derived}: agreement inside the parameter space is weak once metrics that are
derived from one another are removed. The input--parameter block likewise includes zero under
attack clustering ($[-0.41, 0.07]$) while excluding it under configuration and dataset resampling,
which reflects the small number of independent attacks rather than instability of the point
estimate.

\begin{table}[t]
\centering
\scriptsize
\setlength\tabcolsep{3pt}
\caption{Bootstrap $95\%$ confidence intervals for the metric-agreement analysis ($2000$ resamples).
\emph{Config.} resamples individual configurations; \emph{Attack} resamples whole attacks and is the
conservative scheme that respects the dependence between configurations sharing an attack;
\emph{Dataset} resamples whole datasets. Point estimates are identical across schemes by
construction. The within-minus-cross-space gap and the $\ell_1$--TUP association exclude zero under
every scheme; the parameter-space quantities do not survive attack clustering, consistent with
Appendix~\ref{app:rob:derived}.}
\label{tab:app:bootstrap}
\begin{tabular}{@{}l r ccc@{}}
\toprule
\multicolumn{5}{@{}l}{\textbf{All configurations} ($N{=}76$)} \\
\midrule
Quantity & Point & Config. & Attack & Dataset \\
\midrule
Input--Input             & $+0.66$ & $[0.59, 0.72]$ & $[0.43, 0.80]$ & $[0.65, 0.69]$ \\
Feature--Feature         & $+0.57$ & $[0.44, 0.67]$ & $[0.42, 0.65]$ & $[0.32, 0.77]$ \\
Parameter--Parameter     & $+0.27$ & $[0.11, 0.43]$ & $[-0.04, 0.52]$ & $[0.06, 0.55]$ \\
Input--Feature           & $-0.11$ & $[-0.28, 0.06]$ & $[-0.41, 0.24]$ & $[-0.22, 0.05]$ \\
Input--Parameter         & $-0.24$ & $[-0.37, -0.09]$ & $[-0.41, 0.07]$ & $[-0.31, -0.21]$ \\
Feature--Parameter       & $+0.35$ & $[0.24, 0.45]$ & $[0.20, 0.49]$ & $[0.21, 0.53]$ \\
\textbf{Within $-$ cross} & $\mathbf{+0.50}$ & $[0.39, 0.60]$ & $\mathbf{[0.28, 0.62]}$ & $[0.40, 0.61]$ \\
\addlinespace
SS\,$\sim$\,CDBI         & $+0.89$ & $[0.81, 0.92]$ & $[0.81, 0.91]$ & $[0.64, 0.93]$ \\
SS\,$\sim$\,DSWD         & $+0.49$ & $[0.29, 0.65]$ & $[0.31, 0.59]$ & $[0.28, 0.78]$ \\
UCLC\,$\sim$\,TAC        & $+0.05$ & $[-0.22, 0.29]$ & $[-0.44, 0.50]$ & $[-0.13, 0.48]$ \\
$\ell_1$\,$\sim$\,TUP    & $-0.69$ & $[-0.79, -0.54]$ & $\mathbf{[-0.80, -0.47]}$ & $[-0.77, -0.59]$ \\
\midrule
\multicolumn{5}{@{}l}{\textbf{Successful backdoors only}, $\mathrm{ASR}\geq 60\%$ ($N{=}61$)} \\
\midrule
Input--Input             & $+0.69$ & $[0.60, 0.76]$ & $[0.43, 0.82]$ & $[0.67, 0.73]$ \\
Feature--Feature         & $+0.44$ & $[0.29, 0.57]$ & $[0.29, 0.54]$ & $[0.24, 0.68]$ \\
Parameter--Parameter     & $+0.24$ & $[0.05, 0.43]$ & $[-0.07, 0.50]$ & $[-0.00, 0.55]$ \\
Input--Feature           & $-0.11$ & $[-0.28, 0.07]$ & $[-0.43, 0.24]$ & $[-0.19, 0.00]$ \\
Input--Parameter         & $-0.33$ & $[-0.45, -0.17]$ & $[-0.51, 0.06]$ & $[-0.47, -0.26]$ \\
Feature--Parameter       & $+0.29$ & $[0.17, 0.40]$ & $[0.13, 0.43]$ & $[0.16, 0.54]$ \\
\textbf{Within $-$ cross} & $\mathbf{+0.51}$ & $[0.39, 0.61]$ & $\mathbf{[0.27, 0.64]}$ & $[0.44, 0.66]$ \\
\addlinespace
SS\,$\sim$\,CDBI         & $+0.86$ & $[0.74, 0.92]$ & $[0.78, 0.90]$ & $[0.60, 0.92]$ \\
UCLC\,$\sim$\,TAC        & $+0.02$ & $[-0.32, 0.33]$ & $[-0.50, 0.53]$ & $[-0.19, 0.58]$ \\
$\ell_1$\,$\sim$\,TUP    & $-0.72$ & $[-0.82, -0.57]$ & $[-0.82, -0.38]$ & $[-0.84, -0.66]$ \\
\bottomrule
\end{tabular}
\end{table}

\subsection{Repeated Training: Seeds and Target Classes}
\label{app:rob:seeds}

\paragraph{Motivation}
Backdoor training is stochastic in the model initialization, the selection of poisoned samples, the
data ordering and the augmentation, and every attack in the benchmark additionally targets class
$0$. Neither source of variation is visible in a single realization per configuration.

\paragraph{Method}
We retrained BadNets, Blend, WaNet and BppAttack on CIFAR-10 with ResNet18 at a $5\%$ poisoning
rate under five random seeds, and retrained all four attacks against target classes $1$ and $2$,
giving twelve target configurations. Four benign reference models were trained with matching seeds,
since TAC and TUP are defined relative to a benign model trained on the same data; the
target-class variants are seed-$0$ runs and therefore use the published benign reference. All training hyperparameters follow
Appendix~\ref{sec:experimental_settings} exactly; only the seed, or the target class, is varied.

All footprint metrics were then recomputed for every model under a single fixed measurement
protocol: deterministic evaluation transforms, penultimate-layer features extracted under the test
transform, and a t-SNE embedding with a fixed seed and perplexity $30$ for SS and CDBI. TAC and TUP
are computed against the seed-matched benign reference.

\paragraph{A note on comparability}
The recomputation protocol seeds the t-SNE embedding, whereas the values in
Table~\ref{tab:results_feature_resnet18} and Table~\ref{tab:results_newmetric_resnet18} were
produced without a fixed embedding seed. SS and CDBI values in this appendix therefore differ
slightly from the main tables by construction, and only within-appendix comparisons should be made
for those two metrics. As a correctness check, DSWD, UCLC, TAC and TUP --- none of which involve a
stochastic embedding --- reproduce the main tables exactly when the published models are re-measured
under this protocol: for BadNets, UCLC $=6.59$ against $6.59$ in Table~\ref{tab:uclc-tac}; for
Grond, UCLC $=3.60$ and TUP $=1.87$ against $3.60$ and $1.87$; for Adap-Patch, UCLC $=9.91$ and
TUP $=10.2$ against $9.91$ and $10.2$.

\paragraph{Results: effectiveness}
Benign accuracy reproduces closely across seeds for every attack, and ASR for three of the four
(Table~\ref{tab:app:seed_effectiveness}). BadNets, Blend and BppAttack vary by at most $0.2$
points in benign accuracy and $0.1$ points in ASR. WaNet is the exception on both counts: its
benign accuracy spreads by about $3$ points, and \emph{its ASR itself is seed-fragile} ---
$98.5$--$99.8\%$ at three seeds but $63.6\%$ and $75.6\%$ at the other two. On those weak seeds
WaNet's footprints shrink as well (DSWD $1.05$--$1.16$ against $1.8$--$2.2$ on the strong seeds,
TUP $5.5$--$6.6$ against $8.9$--$9.6$): a partially implanted backdoor leaves a smaller trace.
This is the ASR confound of Section~\ref{sec:metric_disagreement} arising spontaneously from the
training seed, and it is why the metric-variation numbers below are reported over all five seeds
rather than over a favourable subset.

\begin{table}[t]
\centering
\scriptsize
\caption{Effectiveness of retrained models across five random seeds (CIFAR-10, ResNet18, $5\%$
poisoning). Values are mean $\pm$ standard deviation over the five runs. BadNets, Blend and
BppAttack retrain reliably; WaNet shows genuine benign-accuracy variance and a seed-fragile ASR
($63.6$--$100\%$).}
\label{tab:app:seed_effectiveness}
\begin{tabular}{@{}l cc cc@{}}
\toprule
Attack & BA (\%) & CV & ASR (\%) & CV \\
\midrule
BadNets   & $94.43 \pm 0.08$ & $0.1\%$ & $100.00 \pm 0.00$ & $0.0\%$ \\
Blend     & $94.31 \pm 0.06$ & $0.1\%$ & $99.80 \pm 0.05$ & $0.05\%$ \\
BppAttack & $94.59 \pm 0.20$ & $0.2\%$ & $99.87 \pm 0.05$ & $0.05\%$ \\
WaNet     & $92.44 \pm 1.34$ & $1.4\%$ & $87.46 \pm 16.85$ & $19.3\%$ \\
\bottomrule
\end{tabular}
\end{table}

\paragraph{Results: metric variation}
Table~\ref{tab:app:seed_metrics} reports every recomputed metric value. The pattern splits by
space. Feature-space metrics and TUP vary moderately across seeds, with median coefficients of
variation of $1.4\%$ (DSWD), $2.9\%$ (SS), $6.0\%$ (CDBI) and $6.9\%$ (TUP); WaNet's weak-ASR
seeds account for most of the upper end. The two parameter-space metrics are substantially
noisier, with median coefficients of variation of $16.6\%$ (UCLC) and $16.5\%$ (TAC), and worst
cases of $26\%$ (WaNet's UCLC) and $36\%$ (WaNet's TAC). We therefore do not claim that
parameter-space \emph{values} are seed-stable. What is stable is the ordering: the rank
correlation of TUP's attack ordering between any two of the five seeds is $\tau = 1.00$ on all
ten pairs, and for TAC the mean is $\tau = 0.67$.

Rank stability is lower for SS, CDBI, DSWD and UCLC (mean $\tau \approx 0.60$, $0.27$, $0.33$,
$-0.07$), but this is largely a consequence of the comparison set rather than of the metrics. The
four attacks in this experiment belong to the same patch/blend and imperceptible families and
their DSWD values span only about $5\%$ on the strong seeds; when four quantities are nearly
tied, small perturbations reorder them and rank correlation collapses. The coefficients of
variation are the informative summary in that regime.

\paragraph{Results: target class}
Attack effectiveness is unaffected by the target class. Benign accuracy and ASR at targets $1$
and $2$ match their target-$0$ values for every attack (BadNets $100\%$ ASR at all three targets,
Blend $99.7$--$99.9\%$, BppAttack $99.6$--$99.8\%$, WaNet $97.6$--$98.5\%$; benign accuracy varies
by at most $0.5$ points). Changing the target class does not make a backdoor easier or harder to
implant.

The effect on the footprint metrics is not uniform, and the division is itself informative.
Table~\ref{tab:app:target_ranks} compares the attack ordering that each metric induces across the
three target classes. SS, DSWD and TUP rank the four attacks identically at every target class,
with median relative value shifts of $3.9\%$, $5.0\%$ and $1.8\%$. CDBI and TAC each exchange a
single adjacent pair. UCLC is the exception: at target class $2$ its ordering bears no relation to
the target-$0$ ordering ($\tau = 0.00$), driven by Blend moving from second-smallest to largest
($6.49$ to $8.46$ --- a shift of the same order as Blend's own five-seed UCLC spread, which is
itself wide: sd $1.6$, inflated by one outlier seed at $10.45$).

We report the UCLC result as a property of that metric rather than of the measurement framework,
because it is consistent with what we observe under seed variation: UCLC is also the least
rank-stable metric across seeds ($\tau \approx -0.1$ over five seeds) and has among the highest
coefficients of variation ($16.6\%$ median, $26\%$ for WaNet), while TUP is the most stable
metric under both perturbations. The same metric is fragile under both, and the same metric is
robust under both. This reinforces the recommendation in
Section~\ref{sec:metric_disagreement} that parameter-space conclusions should not rest on a
single metric: none of the paper's headline results depends on UCLC's ordering alone, since the
parameter-space minimum is identified jointly by UCLC, TAC and TUP, and the attack holding it,
Grond, is itself retrained at all three target classes in Appendix~\ref{app:rob:winners}, where
its parameter-space minimum holds in every run.

The largest single feature-space movement is BppAttack's CDBI, which shifts $24.1\%$ between
target $0$ and target $2$ while leaving the ordering unchanged apart from one adjacent swap. Values
therefore move more than rankings do, which is the same pattern seen across seeds and the reason we
report both.

\begin{table}[t]
\centering
\scriptsize
\setlength\tabcolsep{3.2pt}
\caption{All recomputed footprint measurements for the repeated-training experiment (CIFAR-10,
ResNet18). \emph{Seed 0} rows are the published models re-measured under the recomputation protocol;
\emph{seed 1--4} are independently retrained. \emph{Target 1--2} vary the target class instead of the seed, at seed $0$. SS and CDBI use a seeded t-SNE and are therefore not directly comparable to
Tables~\ref{tab:results_feature_resnet18} and~\ref{tab:results_newmetric_resnet18}; DSWD, UCLC, TAC
and TUP are.}
\label{tab:app:seed_metrics}
\begin{tabular}{@{}ll cc cccccc@{}}
\toprule
Attack & Variant & BA & ASR & SS & CDBI & DSWD & UCLC & TAC & TUP \\
\midrule
\multirow{7}{*}{BadNets}
 & seed 0   & .945 & 1.000 & .448 & .543 & 2.007 & 6.59 & 3.90 & 16.20 \\
 & seed 1   & .944 & 1.000 & .466 & .536 & 2.060 & 7.93 & 3.56 & 14.74 \\
 & seed 2   & .943 & 1.000 & .469 & .550 & 2.041 & 8.44 & 3.67 & 16.98 \\
 & seed 3   & .944 & 1.000 & .447 & .529 & 2.067 & 6.71 & 3.28 & 13.41 \\
 & seed 4   & .945 & 1.000 & .484 & .534 & 2.054 & 6.40 & 3.93 & 13.18 \\
 & target 1 & .946 & 1.000 & .472 & .530 & 2.156 & 6.55 & 3.73 & 16.47 \\
 & target 2 & .945 & 1.000 & .443 & .571 & 2.008 & 6.04 & 3.85 & 16.38 \\
\cmidrule(lr){2-10}
\multirow{7}{*}{Blend}
 & seed 0 & .943 & .998 & .504 & .668 & 2.048 & 6.49 & 3.05 & 3.68 \\
 & seed 1 & .943 & .998 & .499 & .688 & 2.016 & 6.95 & 3.29 & 3.75 \\
 & seed 2 & .943 & .997 & .499 & .645 & 2.055 & 7.19 & 3.64 & 3.61 \\
 & seed 3 & .944 & .998 & .529 & .623 & 2.110 & 7.42 & 4.32 & 3.76 \\
 & seed 4 & .943 & .999 & .506 & .635 & 2.049 & 10.45 & 3.44 & 3.71 \\
 & target 1 & .942 & .999 & .498 & .630 & 2.180 & 6.44 & 4.18 & 3.65 \\
 & target 2 & .944 & .997 & .497 & .661 & 2.017 & 8.46 & 3.07 & 3.61 \\
\cmidrule(lr){2-10}
\multirow{7}{*}{WaNet}
 & seed 0 & .934 & .985 & .419 & .502 & 1.833 & 6.33 & 10.72 & 9.30 \\
 & seed 1 & .917 & .998 & .493 & .706 & 1.913 & 12.08 & 9.74 & 9.62 \\
 & seed 2 & .905 & .998 & .492 & .630 & 2.157 & 7.86 & 14.07 & 8.86 \\
 & seed 3 & .931 & \textbf{.636} & .366 & .686 & 1.055 & 7.29 & 5.19 & 5.54 \\
 & seed 4 & .936 & \textbf{.756} & .391 & .591 & 1.164 & 9.33 & 7.49 & 6.61 \\
 & target 1 & .934 & .976 & .398 & .483 & 1.834 & 6.19 & 11.64 & 9.41 \\
 & target 2 & .929 & .984 & .397 & .504 & 1.797 & 7.43 & 13.81 & 9.46 \\
\cmidrule(lr){2-10}
\multirow{7}{*}{BppAttack}
 & seed 0 & .944 & .998 & .489 & .592 & 1.912 & 9.42 & 8.50 & 21.02 \\
 & seed 1 & .945 & .999 & .488 & .566 & 1.909 & 10.05 & 11.55 & 20.89 \\
 & seed 2 & .946 & .998 & .473 & .598 & 1.917 & 8.22 & 8.18 & 20.94 \\
 & seed 3 & .949 & .998 & .469 & .679 & 1.952 & 10.82 & 7.40 & 20.98 \\
 & seed 4 & .945 & .999 & .488 & .667 & 1.907 & 8.96 & 10.86 & 22.21 \\
 & target 1 & .946 & .998 & .476 & .682 & 1.980 & 8.80 & 7.46 & 20.95 \\
 & target 2 & .945 & .996 & .476 & .734 & 1.902 & 8.07 & 8.94 & 22.22 \\
\midrule
\multicolumn{2}{@{}l}{Median CV across seeds} & \multicolumn{2}{c}{$\leq 0.2\%$} & $2.9\%$ & $6.0\%$ & $1.4\%$ & $16.6\%$ & $16.5\%$ & $6.9\%$ \\
\multicolumn{2}{@{}l}{Rank stability $\tau$ (seed pairs)} & \multicolumn{2}{c}{---} & $0.60$ & $0.27$ & $0.33$ & $-0.07$ & $0.67$ & $\mathbf{1.00}$ \\
\bottomrule
\end{tabular}
\end{table}

\begin{table}[t]
\centering
\scriptsize
\setlength\tabcolsep{3pt}
\caption{Stability of the attack ordering under change of target class. Each metric induces an
ordering of the four attacks; the table reports Kendall's $\tau$ between the orderings obtained at
different target classes, together with the relative movement of the underlying values. SS, DSWD
and TUP are order-preserving; UCLC's ordering does not survive target class $2$. ``Within $2\times$''
counts the attacks whose largest target-induced shift stays inside twice that attack's own
seed-to-seed standard deviation over the five seeds; note that the five-seed spreads are wider than
the three-seed ones (WaNet's weak-ASR seeds in particular), so staying ``within'' spread is the
weaker statement, and UCLC scores $4/4$ here even though its ordering breaks.}
\label{tab:app:target_ranks}
\begin{tabular}{@{}l ccc cc c@{}}
\toprule
& \multicolumn{3}{c}{Kendall $\tau$ between orderings} & \multicolumn{2}{c}{Value shift} & \\
\cmidrule(lr){2-4}\cmidrule(lr){5-6}
Metric & $t_0$--$t_1$ & $t_0$--$t_2$ & $t_1$--$t_2$ & median & max & Within $2\times$ \\
\midrule
SS   & $+1.00$ & $+1.00$ & $+1.00$ & $3.9\%$ & $5.3\%$ & $4/4$ \\
DSWD & $+1.00$ & $+1.00$ & $+1.00$ & $5.0\%$ & $7.4\%$ & $1/4$ \\
TUP  & $+1.00$ & $+1.00$ & $+1.00$ & $1.8\%$ & $5.7\%$ & $3/4$ \\
\addlinespace
CDBI & $+0.67$ & $+0.67$ & $+1.00$ & $5.4\%$ & $24.1\%$ & $2/4$ \\
TAC  & $+0.67$ & $+1.00$ & $+0.67$ & $20.5\%$ & $37.0\%$ & $3/4$ \\
UCLC & $+1.00$ & $\mathbf{0.00}$ & $\mathbf{0.00}$ & $15.8\%$ & $30.3\%$ & $4/4$ \\
\bottomrule
\end{tabular}
\end{table}

\subsection{Re-runs of the Space Winners across Target Classes}
\label{app:rob:winners}

\paragraph{Motivation}
The tri-space conclusion rests on the observation that the smallest measured footprint in each space
belongs to a different attack. Two of those minima --- Adap-Patch in feature space and Grond in
parameter space --- are held by attacks that reach high ASR in comparatively few configurations, so
it is reasonable to ask whether the minima are artifacts of a single fortunate run, or of the fixed
target class.

\paragraph{Method}
Both attacks were retrained fourteen more times from scratch using their original implementations
--- five runs at each of the target classes $0$, $1$ and $2$ --- and all metrics were recomputed
under the protocol of Appendix~\ref{app:rob:seeds}. Every Grond run is fully independent,
generating its own UPGD trigger (which is target-specific) and its own set of poisoned indices, so
the runs capture end-to-end pipeline variance. The Adap-Patch runs vary the training seed and, in
most runs, the sampled poison set as well.

\paragraph{Results}
Table~\ref{tab:app:winners} reports per-target means and spreads over the five runs, and the
resulting separations. Every separation holds in every one of the thirty models: Adap-Patch's
silhouette score never exceeds $0.200$ against a per-target comparison minimum of at least $0.366$
(the target-$0$ minimum is set by a weak-ASR WaNet seed; excluding weak-backdoor models it is
$0.397$), Grond's UCLC never exceeds $4.60$ against at least $6.04$, and Grond's TUP never exceeds
$1.87$ against at least $3.61$. The per-space minima are therefore not artifacts of single fortunate
training runs, nor of the choice of target class.

TUP is again the quietest metric: Grond's per-target TUP means span $1.73$--$1.77$, within its own
run-to-run spread. Grond's UCLC moves with the target class beyond its target-$0$ run spread
(per-target means $3.72$, $4.21$, $3.92$), consistent with UCLC's instability in
Appendix~\ref{app:rob:seeds}, but the movement never approaches the separation boundary. Grond's
silhouette score and CDBI also shift with the target class; neither bears on a headline claim, as
the feature-space minimum is Adap-Patch's. Adap-Patch's ASR is noticeably variable across runs at
\emph{every} target class ($0.71$--$0.97$; per-target means $0.89$, $0.91$, $0.86$) --- run-to-run
variance rather than a target effect --- while its benign accuracy and silhouette score stay put.
Adap-Patch's UCLC remains noisy across runs ($6.4$--$13.5$), but Adap-Patch is among the
\emph{largest} parameter-space footprints in the benchmark, so this variance does not bear on any
claim the paper makes.

\begin{table}[t]
\centering
\scriptsize
\setlength\tabcolsep{3pt}
\caption{Re-runs of the feature- and parameter-space winners at three target classes (CIFAR-10,
ResNet18; five runs per target class, mean $\pm$ sd). \emph{Comparison minimum} is the smallest
value reached by any retrained comparison model at the same target class: the twenty seed-retrained
models of Appendix~\ref{app:rob:seeds} at target $0$, and the four target-retrained models at
targets $1$ and $2$. Every separation holds in every one of the thirty runs.}
\label{tab:app:winners}
\begin{tabular}{@{}ll cccccc@{}}
\toprule
Attack & Target & BA & ASR & SS & UCLC & TAC & TUP \\
\midrule
\multirow{3}{*}{Grond}
 & 0 & $.946{\pm}.003$ & $.978{\pm}.027$ & $.509{\pm}.014$ & $3.72{\pm}0.11$ & $2.93{\pm}0.40$ & $1.73{\pm}0.08$ \\
 & 1 & $.944{\pm}.001$ & $.989{\pm}.003$ & $.363{\pm}.091$ & $4.21{\pm}0.42$ & $2.85{\pm}0.13$ & $1.76{\pm}0.05$ \\
 & 2 & $.950{\pm}.001$ & $.992{\pm}.002$ & $.573{\pm}.008$ & $3.92{\pm}0.52$ & $3.31{\pm}0.24$ & $1.77{\pm}0.03$ \\
\midrule
\multirow{3}{*}{Adap-Patch}
 & 0 & $.943{\pm}.002$ & $.892{\pm}.100$ & $.153{\pm}.037$ & $11.36{\pm}1.74$ & $3.78{\pm}0.63$ & $9.65{\pm}1.28$ \\
 & 1 & $.944{\pm}.001$ & $.906{\pm}.058$ & $.120{\pm}.060$ & $11.06{\pm}2.08$ & $4.49{\pm}0.78$ & $9.46{\pm}0.77$ \\
 & 2 & $.947{\pm}.001$ & $.863{\pm}.068$ & $.107{\pm}.044$ & $10.96{\pm}3.01$ & $3.41{\pm}0.70$ & $9.32{\pm}0.75$ \\
\midrule
\multicolumn{8}{@{}l}{\textbf{Separations (worst run vs.\ comparison minimum at the same target class)}} \\
\midrule
\multicolumn{2}{@{}l}{Adap-Patch SS}
 & \multicolumn{2}{l}{t0: $.200$ vs.\ $.366$ ($1.8\times$)}
 & \multicolumn{2}{l}{t1: $.162$ vs.\ $.398$ ($2.5\times$)}
 & \multicolumn{2}{l}{t2: $.181$ vs.\ $.397$ ($2.2\times$)} \\
\multicolumn{2}{@{}l}{Grond UCLC}
 & \multicolumn{2}{l}{t0: $3.84$ vs.\ $6.33$ ($1.6\times$)}
 & \multicolumn{2}{l}{t1: $4.60$ vs.\ $6.19$ ($1.3\times$)}
 & \multicolumn{2}{l}{t2: $4.57$ vs.\ $6.04$ ($1.3\times$)} \\
\multicolumn{2}{@{}l}{Grond TUP}
 & \multicolumn{2}{l}{t0: $1.87$ vs.\ $3.61$ ($1.9\times$)}
 & \multicolumn{2}{l}{t1: $1.81$ vs.\ $3.65$ ($2.0\times$)}
 & \multicolumn{2}{l}{t2: $1.82$ vs.\ $3.61$ ($2.0\times$)} \\
\bottomrule
\end{tabular}
\end{table}

\subsection{Embedding Sensitivity of CDBI}
\label{app:rob:cdbi}

\paragraph{Motivation}
CDBI is defined through Euclidean distances between group centroids and their scatters, but is
computed on a t-SNE embedding of penultimate-layer features. t-SNE is a non-linear, non
distance-preserving projection with its own random initialization and a perplexity hyperparameter,
so the resulting ranking might reflect the projection rather than the representation it summarizes.

\paragraph{Method}
For each of $54$ configurations --- $18$ per dataset on CIFAR-10, CIFAR-100 and Imagenette --- we
recomputed SS and CDBI in $18$ different representations of the same saved penultimate features:
the raw $512$-dimensional features, PCA projections to $50$ and to $2$ dimensions, and t-SNE at
perplexities $15$, $30$ and $50$ with five random seeds each. This uses the stored features and
requires no retraining. We then compare the attack rankings that each representation induces, using
Spearman correlation between rankings.

\paragraph{Results}
Table~\ref{tab:app:cdbi} reports the outcome. Rankings are insensitive to the t-SNE seed: at every
perplexity and on every dataset, the mean pairwise agreement between rankings produced by two
different seeds is at least $0.93$, and at least $0.98$ on CIFAR-10. This is the direct answer to
the concern that CDBI's ordering reflects the projection's randomness. Averaged over all $153$
pairs of the $18$ representations, including the unprojected raw features, agreement is
$0.84$--$0.94$ depending on dataset, and the sweep recovers the rankings reported in
Table~\ref{tab:results_newmetric_resnet18} at $0.89$--$0.93$.

Absolute values are considerably less stable than rankings: the median relative spread of CDBI
across the fifteen t-SNE runs is $12$--$14\%$. CDBI should therefore be read as a ranking diagnostic
rather than as a quantity comparable in absolute terms across studies, and the embedding seed and
perplexity should be stated whenever it is reported.

Agreement between the t-SNE ranking and the ranking obtained directly from the raw features is
moderate ($0.52$--$0.84$) rather than near-perfect. We therefore claim insensitivity to the
projection \emph{seed} and broad consistency across representations, not that the projection is
irrelevant. Whether CDBI or SS is the more representation-robust of the two is dataset-dependent
--- CDBI is more robust on CIFAR-10, SS on CIFAR-100, and they are equivalent on Imagenette --- so
neither should be preferred on robustness grounds.

\begin{table}[t]
\centering
\scriptsize
\setlength\tabcolsep{4pt}
\caption{Sensitivity of CDBI to the representation it is computed in ($54$ configurations $\times$
$18$ representations). Rankings are stable across t-SNE seeds and recover the published ordering;
absolute values are not stable. SS is shown for comparison.}
\label{tab:app:cdbi}
\begin{tabular}{@{}l ccc c@{}}
\toprule
Quantity (CDBI unless stated) & C10 & C100 & Imagenette & SS (C10) \\
\midrule
t-SNE seed agreement, perplexity $15$ & $0.998$ & $0.982$ & $0.974$ & $1.000$ \\
t-SNE seed agreement, perplexity $30$ & $0.979$ & $0.942$ & $0.987$ & $0.998$ \\
t-SNE seed agreement, perplexity $50$ & $0.995$ & $0.933$ & $0.978$ & $0.995$ \\
\addlinespace
Mean over all $153$ representation pairs & $0.846$ & $0.838$ & $0.939$ & $0.770$ \\
Minimum over all representation pairs & $0.467$ & $0.441$ & $0.827$ & $0.131$ \\
\addlinespace
t-SNE ($p{=}30$) vs.\ raw $512$-d & $0.519$ & $0.529$ & $0.843$ & $0.137$ \\
t-SNE ($p{=}30$) vs.\ PCA-$50$ & $0.536$ & $0.550$ & $0.843$ & $0.137$ \\
t-SNE ($p{=}30$) vs.\ PCA-$2$ & $0.633$ & $0.810$ & $0.915$ & $0.410$ \\
\addlinespace
Agreement with published ranking & $0.921$ & $0.889$ & $0.925$ & $0.897$ \\
Median relative value spread (t-SNE) & $12.4\%$ & $14.0\%$ & $11.8\%$ & $8.2\%$ \\
\bottomrule
\end{tabular}
\end{table}

\subsection{Agreement Excluding Derived Metrics}
\label{app:rob:derived}

\paragraph{Motivation}
Three of the sixteen metrics are derived by construction from others in the suite: PSNR is a
monotone transformation of MSE and is therefore rank-identical to it; CDBI is computed on the same
embedding as SS and shares its geometry; and TUP is built from the same activation differences as
TAC. Their presence could inflate the apparent within-space agreement that
Section~\ref{sec:metric_disagreement} reports, and thereby manufacture part of the
within-versus-across-space contrast.

\paragraph{Method}
We removed PSNR, CDBI and TUP, leaving thirteen metrics (nine input, two feature, two parameter),
and repeated the entire analysis of Appendix~\ref{app:rob:bootstrap} unchanged. With two metrics per
space, the reduced feature and parameter ``blocks'' are single correlations --- SS--DSWD and
UCLC--TAC --- rather than averages, and we report them as such.

\paragraph{Results}
Table~\ref{tab:app:derived} reports the comparison. The concern is partly justified and partly not.
The input block barely changes ($+0.66 \rightarrow +0.63$), confirming that PSNR was redundant but
that the remaining input metrics are not. The feature block decreases moderately
($+0.57 \rightarrow +0.49$). The parameter block collapses from $+0.27$ to $+0.05$, so the internal
agreement previously observed in the parameter space was indeed carried by the shared construction
of TAC and TUP.

The headline contrast nevertheless survives. The within-minus-cross-space gap decreases from
$+0.50$ to $+0.35$, with an attack-cluster interval of $[0.09, 0.52]$ that still excludes zero, and
the three cross-space blocks are essentially unchanged. On the ASR-filtered subset the gap behaves
identically, $+0.51 \rightarrow +0.35$ with interval $[0.07, 0.54]$.

We read the collapse of the parameter block as strengthening rather than weakening the paper's
thesis. UCLC and TAC were designed independently, by different authors, to capture downstream
channel influence and trigger-induced activation change respectively. That two such metrics agree at
$\rho \approx 0.05$ when pooled is the most direct available evidence that footprint metrics are not
interchangeable even within a single observation space. Pooling does contribute to the effect ---
computed within each dataset and averaged, UCLC--TAC agreement is $+0.44$, reflecting the very
different activation scales across datasets --- and the block-level counterpart of this contrast
($+0.50$ within-dataset versus $+0.27$ pooled) appears in
Table~\ref{tab:metric_correlation_blocks}; both pair-level figures are reported here.

\begin{table}[t]
\centering
\scriptsize
\setlength\tabcolsep{3pt}
\caption{Metric agreement with and without the three metrics that are derived by construction from
others (PSNR, CDBI, TUP). Intervals are attack-cluster bootstrap $95\%$ intervals. The
within-versus-cross contrast survives; the parameter block does not, which sharpens rather than
contradicts the paper's claim that footprint metrics are not interchangeable.}
\label{tab:app:derived}
\begin{tabular}{@{}l cc cc@{}}
\toprule
 & \multicolumn{2}{c}{Full suite ($16$)} & \multicolumn{2}{c}{Reduced ($13$)} \\
\cmidrule(lr){2-3}\cmidrule(lr){4-5}
Quantity & Point & CI & Point & CI \\
\midrule
Input--Input          & $+0.66$ & $[0.43, 0.80]$ & $+0.63$ & $[0.40, 0.80]$ \\
Feature--Feature      & $+0.57$ & $[0.42, 0.65]$ & $+0.49$ & $[0.31, 0.59]$ \\
Parameter--Parameter  & $+0.27$ & $[-0.04, 0.52]$ & $+0.05$ & $[-0.43, 0.50]$ \\
Input--Feature        & $-0.11$ & $[-0.41, 0.24]$ & $-0.07$ & $[-0.36, 0.25]$ \\
Input--Parameter      & $-0.24$ & $[-0.41, 0.07]$ & $-0.16$ & $[-0.36, 0.20]$ \\
Feature--Parameter    & $+0.35$ & $[0.20, 0.49]$ & $+0.34$ & $[0.17, 0.51]$ \\
\textbf{Within $-$ cross} & $\mathbf{+0.50}$ & $[0.28, 0.62]$ & $\mathbf{+0.35}$ & $\mathbf{[0.09, 0.52]}$ \\
\addlinespace
\multicolumn{5}{@{}l}{$\mathrm{ASR}\geq 60\%$ subset} \\
\textbf{Within $-$ cross} & $+0.51$ & $[0.27, 0.64]$ & $+0.35$ & $[0.07, 0.54]$ \\
Parameter--Parameter & $+0.24$ & $[-0.07, 0.50]$ & $+0.02$ & $[-0.51, 0.52]$ \\
\bottomrule
\end{tabular}
\end{table}

\subsection{Summary}
\label{app:rob:summary}

Across the four analyses, the paper's structural conclusions are stable and its quantitative
conclusions are stable to the extent claimed.

\begin{itemize}
\item The within-versus-across-space agreement contrast survives resampling at the level of whole
      attacks, survives the exclusion of failed backdoors, and survives the removal of every metric
      derived by construction from another. In every case the interval excludes zero.
\item Excluding low-ASR configurations \emph{strengthens} the central input--parameter disagreement,
      from $-0.24$ to $-0.33$.
\item Feature-space metrics and TUP vary by $1$--$7\%$ across training seeds; UCLC and TAC vary by
      ${\sim}17\%$. Parameter-space \emph{orderings} are stable where the values are not, with TUP's
      ordering fully seed-invariant.
\item Each per-space minimum is retained under every retrained model, including independent re-runs
      of both attacks whose minima rest on the fewest successful configurations.
\item Varying the target class leaves attack effectiveness unchanged and preserves the attack
      ordering exactly for SS, DSWD and TUP. CDBI and TAC each exchange one adjacent pair, and
      UCLC's ordering does not survive target class $2$ --- the same metric that is least stable
      across seeds, and a reason not to rest parameter-space conclusions on a single metric.
\item CDBI's attack rankings are insensitive to the t-SNE seed and broadly consistent across
      eighteen representations, while its absolute values are not; it should be reported as a
      ranking diagnostic with a stated embedding.
\end{itemize}

Two limitations of this appendix should be stated plainly. First, repeated training covers six
attacks on one dataset and one architecture, not the full benchmark; the bootstrap analyses, which
do cover all $76$ configurations, are what generalize. Second, agreement between UCLC and TAC is
weak once derived metrics are removed, so parameter-space conclusions in this paper rest on the
individual metrics and their agreement on the identity of the quietest attack, not on the parameter
block behaving as a coherent aggregate.
